# Supplementary material for: Dicke states as matrix product states
Source: arXiv:2408.04729 source file (2024-11-23)
Supplement: Supplementary file 1 [file MPS_Dicke_arxiv2.pdf]

# Sequential deterministic preparation of Dicke states $|D_k^n\rangle$

Upload this notebook to https://colab.research.google.com

```
try:
    import cirq
except ImportError:
    print("installing cirq...")
    !pip install --quiet cirq
    import cirq

    print("installed cirq.")
```

```
installing cirq...
     ━━━━━━━━━━━━━━━━━━━━━━━━━━━━━━━━━━━━━━━━ 45.6/45.6 kB 1.6 MB/s eta 0:00:00
  Preparing metadata (setup.py) ... done
   ━━━━━━━━━━━━━━━━━━━━━━━━━━━━━━━━━━━━━━━━ 1.9/1.9 MB 34.1 MB/s eta 0:00:00
   ━━━━━━━━━━━━━━━━━━━━━━━━━━━━━━━━━━━━━━━━ 532.7/532.7 kB 25.0 MB/s eta 0:00:00
   ━━━━━━━━━━━━━━━━━━━━━━━━━━━━━━━━━━━━━━━━ 60.5/60.5 kB 4.2 MB/s eta 0:00:00
   ━━━━━━━━━━━━━━━━━━━━━━━━━━━━━━━━━━━━━━━━ 69.3/69.3 kB 5.1 MB/s eta 0:00:00
   ━━━━━━━━━━━━━━━━━━━━━━━━━━━━━━━━━━━━━━━━ 596.5/596.5 kB 27.9 MB/s eta 0:00:00
   ━━━━━━━━━━━━━━━━━━━━━━━━━━━━━━━━━━━━━━━━ 202.6/202.6 kB 14.2 MB/s eta 0:00:00
   ━━━━━━━━━━━━━━━━━━━━━━━━━━━━━━━━━━━━━━━━ 6.8/6.8 MB 69.5 MB/s eta 0:00:00
   ━━━━━━━━━━━━━━━━━━━━━━━━━━━━━━━━━━━━━━━━ 53.0/53.0 kB 3.4 MB/s eta 0:00:00
   ━━━━━━━━━━━━━━━━━━━━━━━━━━━━━━━━━━━━━━━━ 2.0/2.0 MB 59.0 MB/s eta 0:00:00
   ━━━━━━━━━━━━━━━━━━━━━━━━━━━━━━━━━━━━━━━━ 1.7/1.7 MB 55.8 MB/s eta 0:00:00
   ━━━━━━━━━━━━━━━━━━━━━━━━━━━━━━━━━━━━━━━━ 117.8/117.8 kB 8.2 MB/s eta 0:00:00
   ━━━━━━━━━━━━━━━━━━━━━━━━━━━━━━━━━━━━━━━━ 526.7/526.7 kB 29.6 MB/s eta 0:00:00
  Building wheel for rpcq (setup.py) ... done
installed cirq.
```

```
import numpy as np
```

# Basic qudit gates

```
simulator = cirq.Simulator()
```

```
class ominus(cirq.Gate):
  def __init__(self, k):
    super(ominus, self)
    self.k = k
  def _qid_shape_(self):
    return (k+1,)
  def _unitary_(self):
    v=np.ones((k,), dtype=int)
    mat=np.diag(v,1)
    mat[k,0]=1
    return mat
  def _circuit_diagram_info_(self, args):
    return f"ominus"

class oplus(cirq.Gate):
  def __init__(self, k):
    super(oplus, self)
    self.k = k
  def _qid_shape_(self):
    return (k+1,)
  def _unitary_(self):
    v=np.ones((k,), dtype=int)
    mat=np.diag(v,-1)
    mat[0,k]=1
    return mat
  def _circuit_diagram_info_(self, args):
    return f"oplus"
```

## Circuit for preparing $|D_k^n\rangle|k\rangle$

```
def gamma(n,k,i,l):
  if k-l<=n-i+1:
    return np.sqrt(1+((l-k)/(n-i+1)))
  else:
    return 0


def Igate(qr,qra,n,k,i,l):
  theta=2*np.arccos(gamma(n,k,i,l))
  coplus=cirq.ControlledGate(oplus(k),num_controls=1, control_values=(0,),\
                             control_qid_shape=(2,))
  cominus=cirq.ControlledGate(ominus(k),num_controls=1, control_values=(0,),\
                             control_qid_shape=(2,))
  cr = cirq.ControlledGate(cirq.ry(theta),num_controls=1,\
                           control_values=((l+1) % (k+1),),\
                             control_qid_shape=(k+1,))
  yield coplus(qr[i-1],qra)
  yield cr(qra,qr[i-1])
  yield cominus(qr[i-1],qra)

#simplified!
def Ugate(qr,qra,n,k,i):
  for l in range(max(0,i-n+k-1),min(i,k)):
    yield Igate(qr,qra,n,k,i,l)

def U(qr,qra,n,k):
  for i in range(1,n+1):
    yield Ugate(qr,qra,n,k,i)
```

## Examples

Note that the bottom wire in the circuit diagram is a qudit (d=k+1), and appears rightmost in the statevector.

```
n=4
k=2
qr=cirq.LineQid.range(n, dimension=2)
qra=cirq.NamedQid('a',dimension=k+1)
test=cirq.Circuit(U(qr,qra,n,k))
print(test)
```

```
0 (d=2): ───(0)───Ry(0.5π)───(0)──────────────────────────────────────────────────────────────────────────────────────
            │     │          │
1 (d=2): ───┼─────┼──────────┼───(0)───Ry(0.608π)───(0)───(0)───Ry(0.392π)───(0)──────────────────────────────────────
            │     │          │   │     │            │     │     │            │
2 (d=2): ───┼─────┼──────────┼───┼─────┼────────────┼─────┼─────┼────────────┼───(0)───Ry(π)───(0)───(0)───Ry(
            │     │          │   │     │            │     │     │            │   │     │        │     │     │
3 (d=2): ───┼─────┼──────────┼───┼─────┼────────────┼─────┼─────┼────────────┼───┼─────┼────────┼─────┼─────┼
            │     │          │   │     │            │     │     │            │   │     │        │     │     │
a (d=3): ───oplus─@──────────ominus──oplus─@────────ominus──oplus─(2)────────ominus──oplus─@────ominus──oplus─(2)
```

```
result = simulator.simulate(test)
print(cirq.dirac_notation(result.final_state_vector, qid_shape=(2,)*n+(k+1,)))
```

```
0.41|00112⟩ + 0.41|01012⟩ + 0.41|01102⟩ + 0.41|10012⟩ + 0.41|10102⟩ + 0.41|11002⟩
```

```
n=5
k=2
qr=cirq.LineQid.range(n, dimension=2)
qra=cirq.NamedQid('a',dimension=k+1)
test=cirq.Circuit(U(qr,qra,n,k))
print(test)
```

```
0 (d=2): ───(0)───Ry(0.436π)───(0)────────────────────────────────────────────────────────────────────────────────────
            │     │            │
1 (d=2): ───┼─────┼────────────┼───(0)───Ry(0.5π)───(0)───(0)───Ry(0.333π)───(0)──────────────────────────────────────
            │     │            │   │     │          │     │     │            │
2 (d=2): ───┼─────┼────────────┼───┼─────┼──────────┼─────┼─────┼────────────┼───(0)───Ry(0.608π)───(0)───(0)───
```

```
          │        │             │       │       │          │        │       │            │        │       │            │
3 (d=2): ─┼────────┼─────────────┼───────┼───────┼──────────┼────────┼───────┼────────────┼────────┼───────┼────────────┼────────┼──
          │        │             │       │       │          │        │       │            │        │       │            │
4 (d=2): ─┼────────┼─────────────┼───────┼───────┼──────────┼────────┼───────┼────────────┼────────┼───────┼────────────┼────────┼──
          │        │             │       │       │          │        │       │            │        │       │            │
a (d=3): ──oplus───@─────────────ominus──oplus───@──────────ominus───oplus───(2)──────────ominus───oplus───@────────────ominus───oplus─
```

```
result = simulator.simulate(test)
print(cirq.dirac_notation(result.final_state_vector, qid_shape=(2,)*n+(k+1,)))
```

```
0.32|000112⟩ + 0.32|001012⟩ + 0.32|001102⟩ + 0.32|010012⟩ + 0.32|010102⟩ + 0.32|011002⟩ + 0.32|100012⟩ + 0.32|100102⟩ + 0.32|101002⟩ + 0.32
```

```
n=6
k=3
qr=cirq.LineQid.range(n, dimension=2)
qra=cirq.NamedQid('a',dimension=k+1)
test=cirq.Circuit(U(qr,qra,n,k))
print(test)
```

```
0 (d=2): ───(0)──────Ry(0.5π)───(0)───────────────────────────────────────────────────────────────────────────────────────────────────
            │        │          │
1 (d=2): ───┼────────┼──────────┼───────(0)──────Ry(0.564π)───(0)───────(0)──────Ry(0.436π)───(0)─────────────────────────────────────
            │        │          │       │        │            │         │        │            │
2 (d=2): ───┼────────┼──────────┼───────┼────────┼────────────┼─────────┼────────┼────────────┼───────(0)──────Ry(0.667π)───(0)───────(0)──
            │        │          │       │        │            │         │        │            │       │        │            │         │
3 (d=2): ───┼────────┼──────────┼───────┼────────┼────────────┼─────────┼────────┼────────────┼───────┼────────┼────────────┼─────────┼──
            │        │          │       │        │            │         │        │            │       │        │            │         │
4 (d=2): ───┼────────┼──────────┼───────┼────────┼────────────┼─────────┼────────┼────────────┼───────┼────────┼────────────┼─────────┼──
            │        │          │       │        │            │         │        │            │       │        │            │         │
5 (d=2): ───┼────────┼──────────┼───────┼────────┼────────────┼─────────┼────────┼────────────┼───────┼────────┼────────────┼─────────┼──
            │        │          │       │        │            │         │        │            │       │        │            │         │
a (d=4): ───oplus────@──────────ominus──oplus────@────────────ominus────oplus────(2)──────────ominus──oplus────@────────────ominus────oplus─
```

```
result = simulator.simulate(test)
print(cirq.dirac_notation(result.final_state_vector, qid_shape=(2,)*n+(k+1,)))
```

```
0.22|0001113⟩ + 0.22|0010113⟩ + 0.22|0011013⟩ + 0.22|0011103⟩ + 0.22|0100113⟩ + 0.22|0101013⟩ + 0.22|0101103⟩ + 0.22|0110013⟩ + 0.22|01101
```

Start coding or generate with AI.
